# Supplementary material for: Non-linear hybrid surface-defect states in defective Bi$_2$Se$_3$
Source: arXiv:2201.03320 ancillary file (2022-07-21)
Supplement: Supplementary file 1 [file supplementary.pdf]

# Supporting Information
## Non-linear Hybrid Surface-defect States In Defective $Bi_2Se_3$

Sharmila N. Shirodkar[1] and Pratibha Dev[1]

[1]*Department of Physics and Astronomy, Howard University, Washington D.C. 20059, United States*

July 5, 2022

# Contents

**S1 Surface states in 1×1×6 QL pristine slab** **S2**

**S2 Inversion symmetric Se vacancies in 5×5×7 QLs slab** **S3**

S2.1 Electronic bandstructure . . . . . . . . . . . . . . . . . . . . . . . . . . . . . . . S3

S2.2 Wavefunctions . . . . . . . . . . . . . . . . . . . . . . . . . . . . . . . . . . . . . S4

S2.3 STM images . . . . . . . . . . . . . . . . . . . . . . . . . . . . . . . . . . . . . . S7

**S3 Band structure plots: wide energy range** **S8**

**S4 Wavefunctions at M-point for $VSe_1$, $VSe_1$' and $VSe_2$** **S8**

**S5 Bandstructure with and without spin-orbit effects** **S9**

**S6 Defect bands in $VSe1_s$** **S9**

**S7 Numerical model for $VSe1_s$** **S10**

**S8 Spin-momentum locking plots** **S11**

**S9 Depolarizing field across the defective slab** **S12**

**S10 Rashba splitting in $VSe_1$** **S13**

**S11 Convergence plots** **S14**

**S12 $VSe1_s$ in 3×3×7, 5×5×7 and 6×6×6 QL slabs** **S15**

## S1 Surface states in 1×1×6 QL pristine slab

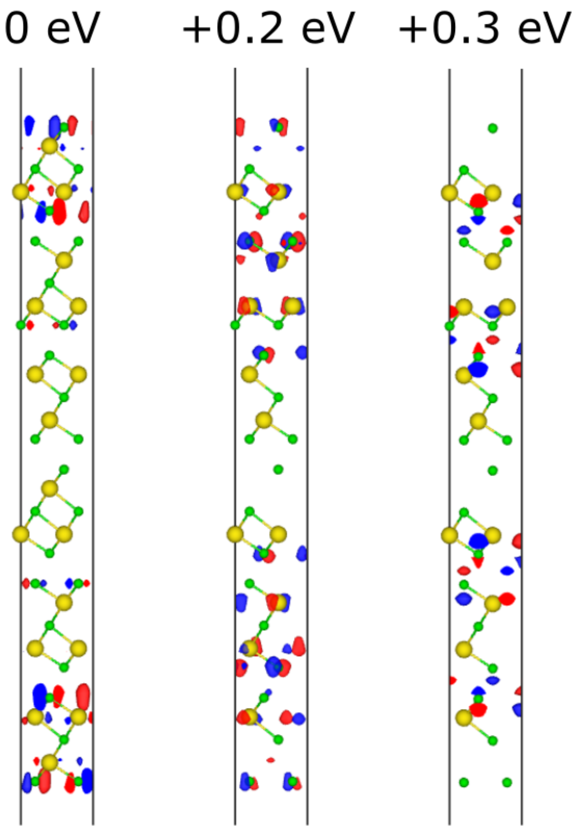


Figure S1: Wavefunctions of in 1×1×6 QL slab at the Γ-point in the BZ. The energy of the state with respect to Fermi level is indicated above the respective wavefunction plots. Note that each wavefunction state is doubly degenerate. Color scheme, Se: green and Bi: yellow. The opposite phases of the wavefuctions are denoted by red and blue colors in the charge density plots.

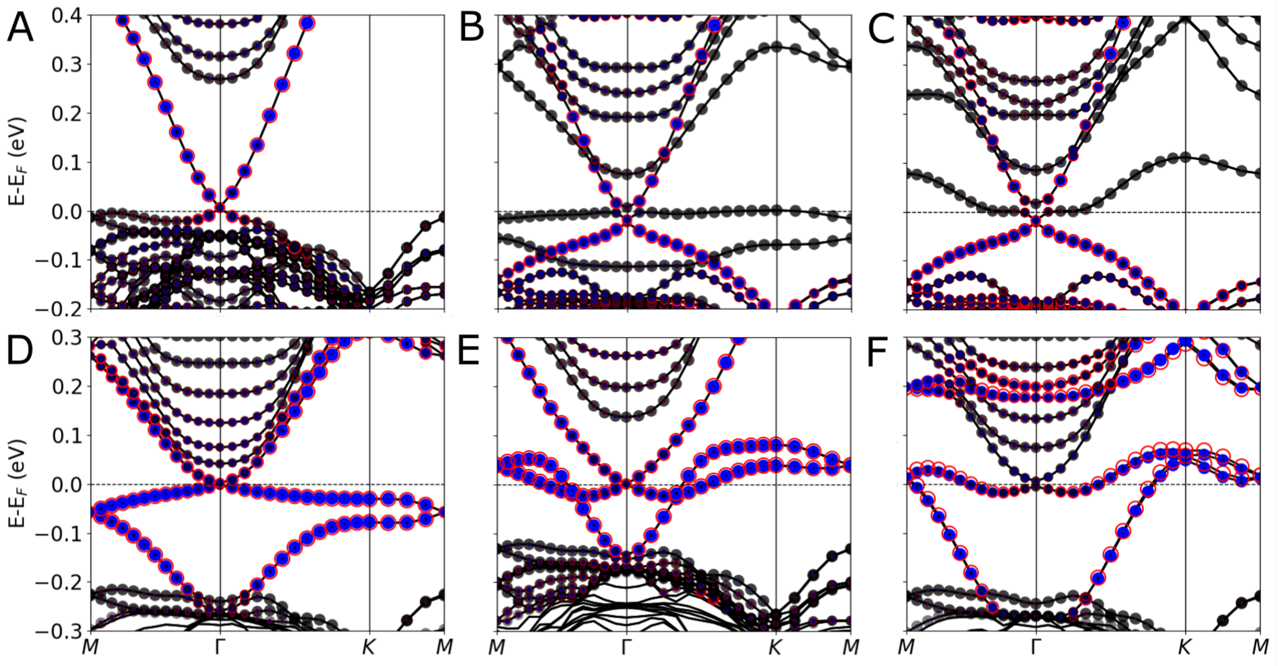


Figure S2: Electronic structure of 5×5×7 QL supercell slab with bulk (top row) and surface (bottom row) Se vacancies. Panels are as follows, A) pristine structure, B) VSe1$_b$, and C) VSe2$_b$; D) VSe1$_s$, E) VSe1$_s$'and F) VSe2$_s$. Note that there is only one vacancy in the case of VSe2$_b$ as opposed to 2 in the rest of the cases. Color scheme, red: top QL contribution, blue: bottom QL contribution and black: bulk contribution to the electronic states. The red circles are made larger to stand out.

# S2 Inversion symmetric Se vacancies in 5×5×7 QLs slab

We create symmetric vacancies that don't break the degeneracy of the top and bottom surfaces in the 5×5×7 QLs slab. Therefore there are a pair of Se vacancies in each VSe1$_b$, VSe1$_s$, VSe1$_s$'and VSe2$_s$ configurations, with the exception of VSe2$_b$ which has only one Se vacancy. This corresponds to a defect concentration of $\approx 10^{19}$ cm$^{-3}$ (in-plane concentration $= 2.6 \times 10^{13}$ cm$^{-2}$), as compared to the reported experimental defect concentrations of about $10^{11}$ to $10^{20}$ cm$^{-3}$ [1, 2]. All the configurations were relaxed without spin-orbit coupling (refer to Methods section, in the main text for details) and the electronic structure analysis was carried out on the relaxed structures with the inclusion of spin-orbit coupling effects. We also consider the effect of charged defects on their stability and find that negatively charged VSes are the most stable in Bi rich conditions (see S4 for details).

## S2.1 Electronic bandstructure

The electronic bandstructures of all the vacancy configurations are shown in Figure S2B-F, with red (blue) circles representing the top (bottom) surface (QL) contribution to the electronic states and black being the contribution of the bulk. In all the cases we note that the inversion symmetry is reflected in the degeneracy of the top and bottom Dirac cones states. Except for some differences, we find that the overall qualitative behavior of the bands is similar to that

of asymmetric defects in 6×6×6 QLs slab. It is important to note that each state at the Γ and M-points in the Brillouin Zone is doubly degenerate, preserving the topological nature of $Bi_2Se_3$.

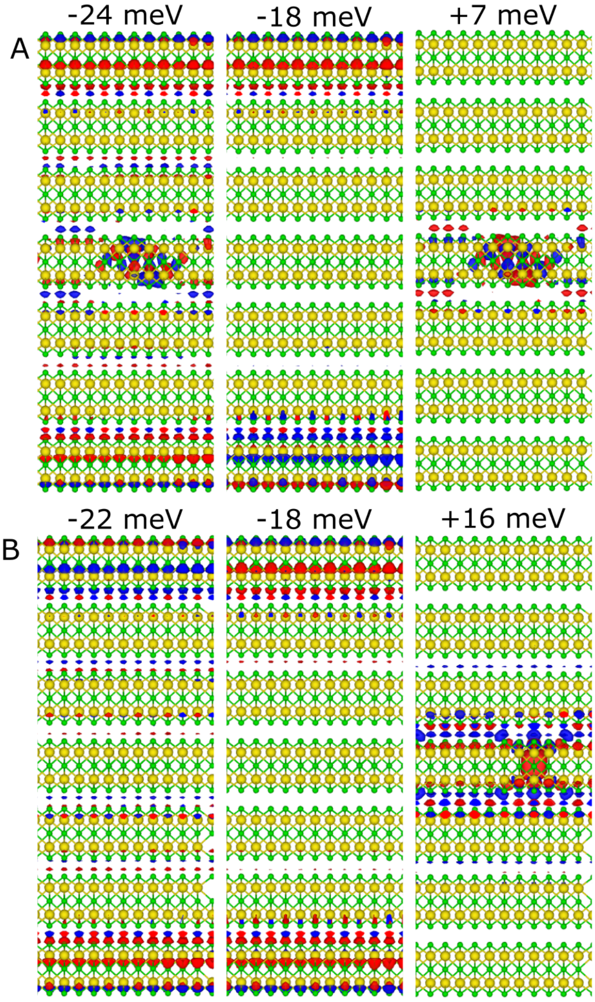


Figure S3: Wavefunctions of bulk Se vacancies in 5×5×7 QL slab at the Γ-point in the BZ. Top row A) is for $VSe1_b$ and bottom row B) is for $VSe2_b$. The energy of the state with respect to Fermi level is indicated above the respective wavefunction plots. Note that each wavefunction state is doubly degenerate. Color scheme, Se: green and Bi: yellow.

## S2.2 Wavefunctions

The artificial symmetry in the defects introduces increased complexity in the band structure and the wavefunctions as compared with 6×6×6 QLs slab. We find that the surface states at both, top and bottom QL couple strongly, giving rise to states with wavefunctions localized to both the layers (see Figures S3 A and B, first and middle column). These states have the same character but are non-degenerate, which is a consequence of this added symmetry. In the case of bulk Se vacancies, we find the surface states to be shifted to ≈ -24 to -18 meV below the Fermi level. The slight foray of the surface states deeper into the slab is on account of interaction between the top and bottom layers with the defect due to finite slab thickness [3] (explained in main text). For a considerably thick slab, the interaction between the defect and

the surface states should be negligible and hence the shift too. Similar to the 6×6×6 QLs slab, $VSe2_b$ decouples from the surface states (at ≈ -22 meV and -18 meV below the Fermi level). The defect state can be seen clearly in the conduction band at ≈ +7 meV and +16 meV, for $VSe1_b$ and $VSe2_b$, respectively.

For $VSe1_s$, we find hybrid topological states (defect + surface states) around the Γ-point only, with no deeper surface states detected even for energies as low as -650 meV. These hybrid states are further connected to the bulk-like state at about -240 meV (see Figure S4 A, leftmost panel). We attribute this behavior, which appears to be different from that seen in asymmetric $VSe1_s$-defect in 6×6×6 QLs slab to an increased interactions between defect and surface states, as well as between the surfaces (across the slab) in $VSe1_s$ case, since it lies at the interface of vacuum and the topological insulator.

The degeneracy between the top and bottom surface states is preserved by the inversion-symmetric placement of surface Se vacancies (see Figure S4, first-column). The surface states for $VSe1_s$' and $VSe2_s$ shift by ≈ -153 meV and -440 meV below the Fermi level (see Figure S4 B and C).The states at the Fermi level (see Figure S4 middle and right-most columns), mostly show defect character. They arise from the hybridization between the top and bottom surface states and the defect state (see main text for detailed explanation). However, due to the symmetry of the defects, each of these states below and above the Fermi level are a result of the mixing between the a) doubly degenerate pair surface states and b) the defect state. Since the defect is an integral part of the top and bottom QL layers, its signature is prominent in these states (as in the case of 6×6×6 QLs slab in main text).

To further explore why we do not have a mostly defect-like hybrid state around Fermi level and a mostly surface-like hybrid state deeper in the valence band in the case of $VSe1_s$, we carry out calculations for a single Se vacancy at the top surface (see Figure S5). As expected the electronic band structure (see Figure S5 A) of the top surface (red) shows exactly the same behaviour as $VSe1_s$ in 6×6×6 QLs slab. This is confirmed by the observation of the top surface Dirac cone at ≈ -275 meV, bottom surface Dirac cone at ≈ -5 meV, and the symmetrically split defect state at ≈ +5 meV (see Figure S5 B).

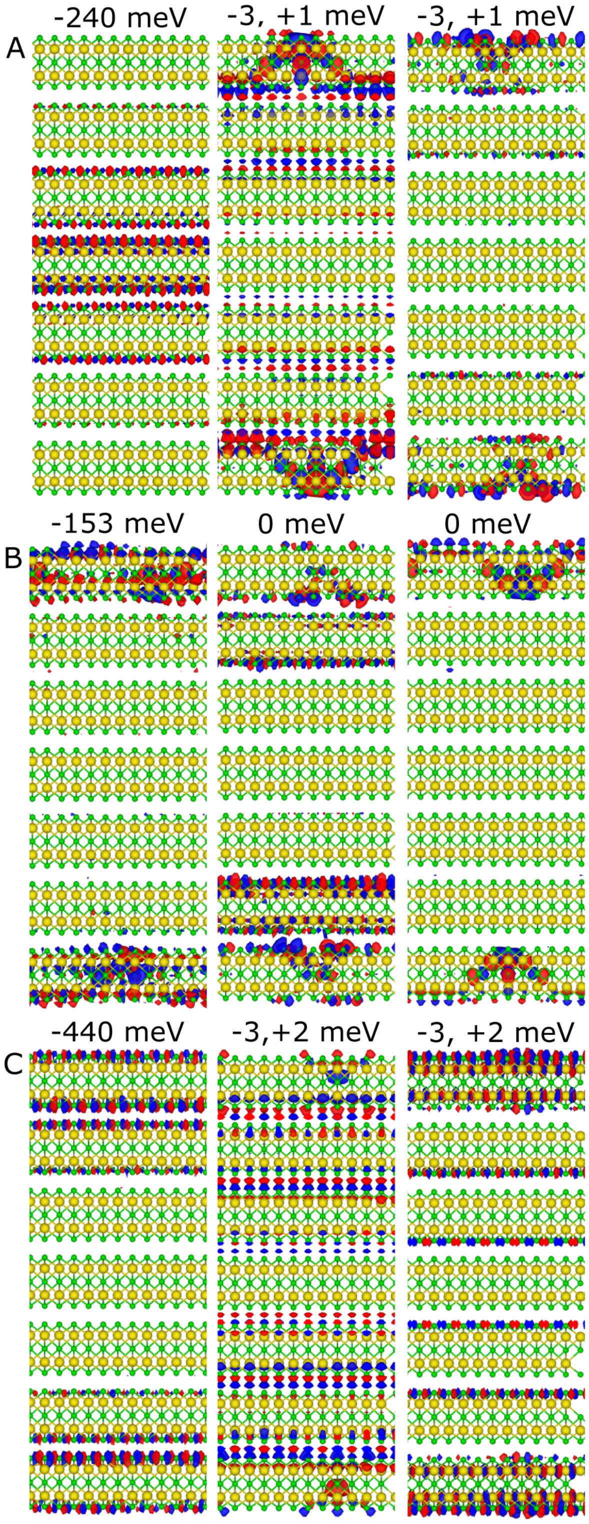


Figure S4: Wavefunctions of Se vacancies on the surface of 5×5×7 QL slab at the Γ-point in the BZ. Top row A) is for $VSe1_s$, middle row B) is for $VSe1_s$' and bottom row C) is for $VSe2_s$. The energy of the state with respect to Fermi level is indicated above the respective wavefunction plots. Note that each wavefunction state is doubly degenerate; and for A) and C), an additional mixing of states at the Fermi level (middle and last columns) is observed due to the imposed inversion symmetry and leads to mixing of the doubly degenerate pair surface states with defect states. Color scheme, Se: green and Bi: yellow.

## S2.3 STM images

The STM signatures of the 3 surface vacancy configurations are given in Figure S5.The STM images are produced at a constant height above the top Se layer at V= +1 V i.e. they sample the conduction band. $VSe1_s$ can be distinguished by the dark spot in it's STM image, whereas $VSe1_s$'is located at the center of the intersection of three dark and light triangles. $VSe2_s$ is the most indistinct with no clear signature.

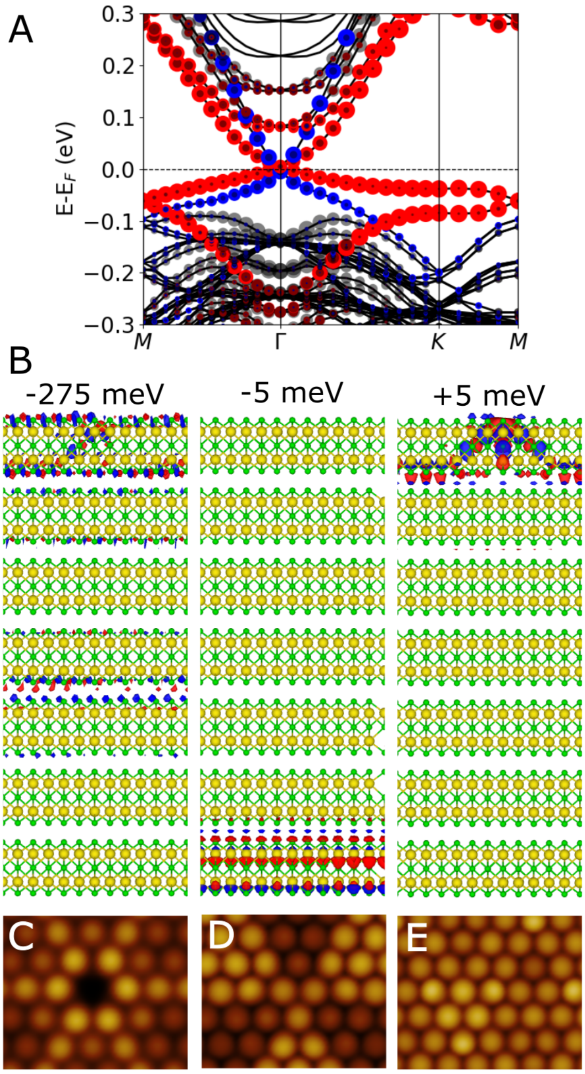


Figure S5: Electronic band structure and wavefunctions of 1 $VSe_s$ and simulated STM images of all the surface vacancies at the top surface of 5×5×7 QL slab. A) shows the band structure, with color scheme, red: top QL contribution, blue: bottom QL contribution and black: bulk contribution to the electronic states. B) shows the wavefunctions with energy of the state with respect to Fermi level indicated above the respective wavefunction plots. Constant height STM images of vacancies, C) $VSe1_s$, D) $VSe1_s$' and E) $VSe2_s$ are produced at a constant height above the top Se layer for V= +1 V. Note that each wavefunction state is doubly degenerate. Color scheme, Se: green and Bi: yellow.

# S3 Band structure plots: wide energy range

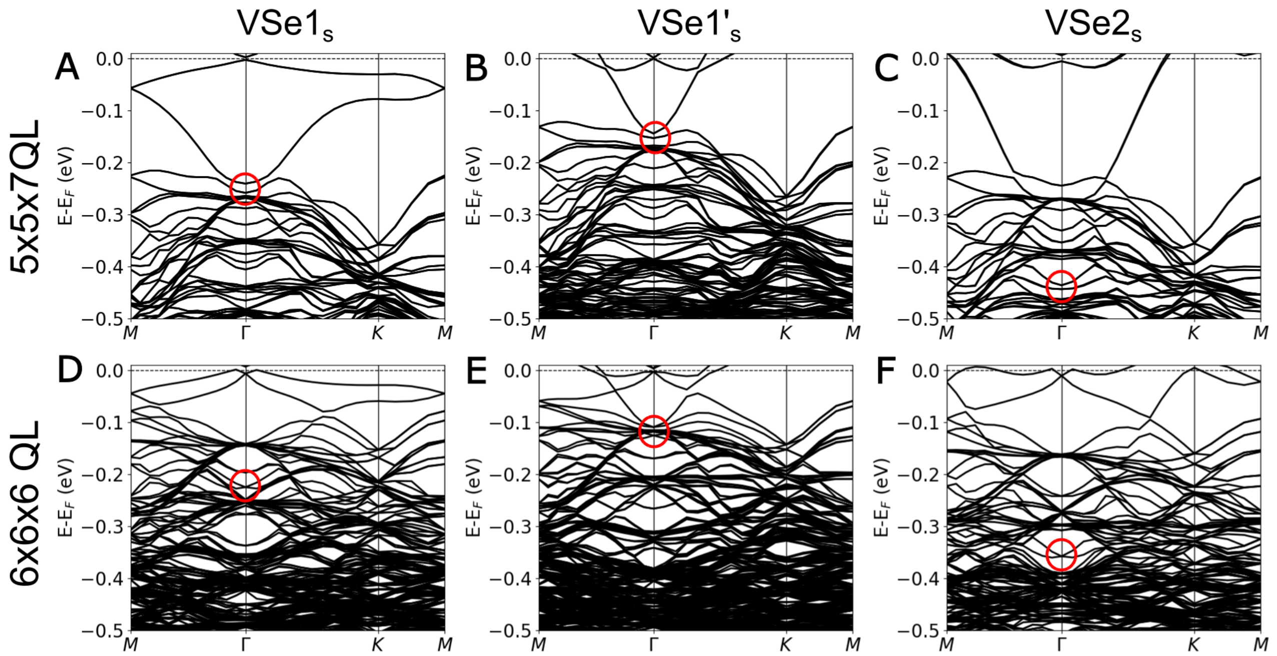


Figure S6: Electronic band structure deeper into the valence band for surface Se vacancies in both, 5×5×7 QL (top row) and 6×6×6 QL slabs (bottom row). The energy at which surface states are observed is denoted by red circles.

# S4 Wavefunctions at M-point for $VSe_1$, $VSe_1$' and $VSe_2$

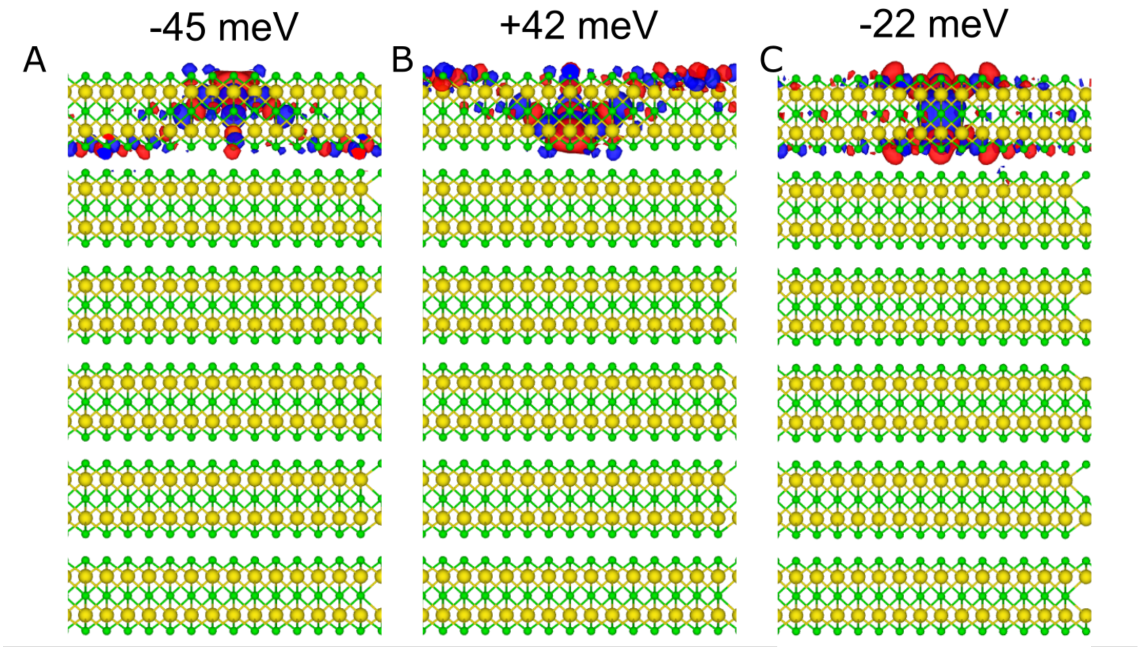


Figure S7: Wavefunctions at the M-point for $VSe_s$ in 6×6×6 QLs slab, denoted by * in main text Figure 3 A, C and E. The charge densities of the wavefunctions are shown in A) for $VSe1_s$, B) for $VSe1_s$' and C) for $VSe2_s$. Color scheme, Se: green and Bi: yellow. The opposite phases of the wavefuctions are denoted by red and blue colors.

# S5 Bandstructure with and without spin-orbit effects

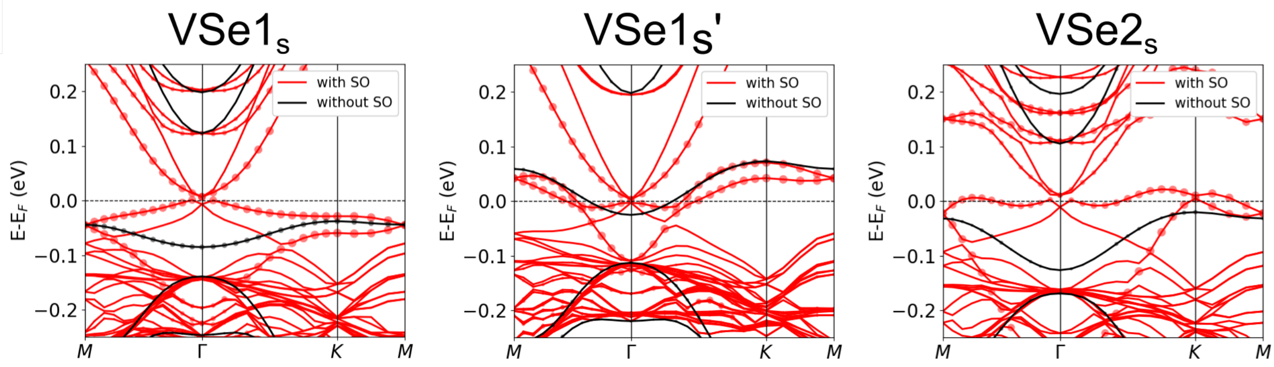


Figure S8: Comparison of the band structure of VSe$1_s$ with (red) and without (black) spin-orbit coupling (SO) effects. The top QL (with defect) contributions are shown in circles. Note that the VBM and CBM of calculations without SO are scissors shifted to match the ones with SO to aid the comparison.

In the absence of spin-orbit coupling, the defect band is almost flat and partially filled, but with the inclusion of spin-orbit effects it mixes with the top QL surface state and shows spin-splitting. One spin branch shows high upward dispersion (parabolic-like) with band minimum pinned close to the Fermi level (see Figure S8); unlike the 2DEG [4–7] which exists higher in the conduction band. While the other spin branch mixes with the surface state and disperses below the Fermi level, with the Dirac cone shifting deep inside the valence band as explained in the main text.

# S6 Defect bands in VSe$1_s$

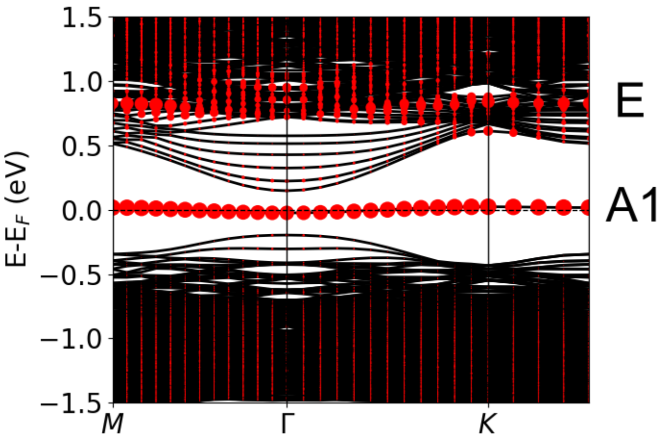


Figure S9: Electronic band structure of VSe$1_s$ with the contribution of Bi atom surrounding the Se vacancy shown in red, without the spin-orbit coupling (SO) effects.

VSe$1_s$ defect has the 3m point group symmetry. The defect bands thus have A1 and E irreducible symmetry representation, and are labeled in the figure.

## S7 Numerical model for VSe$1_s$

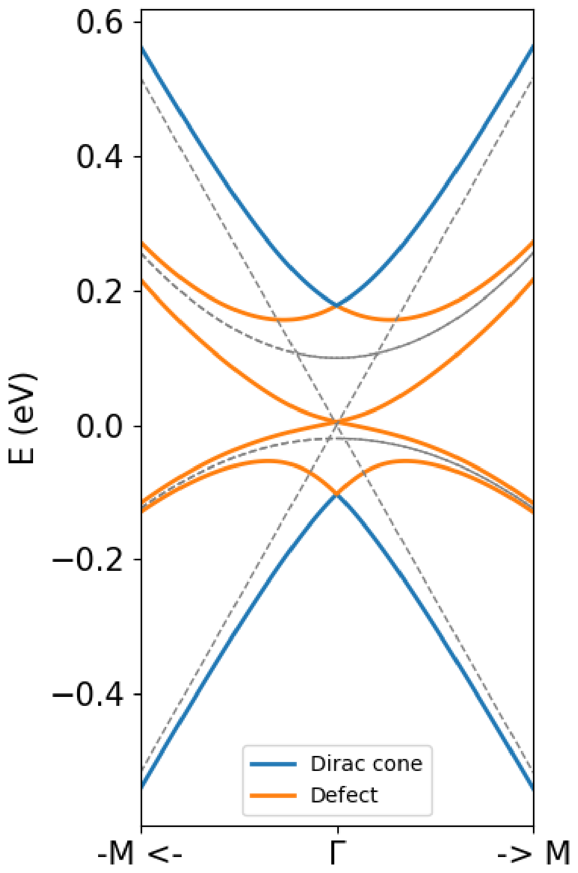


Figure S10: Numerical model of hybridization [8] between the Dirac cone (blue), and the defect and QW states (orange). Dashed grey lines represent the states are before switching on the interaction. We have used $v_F = 5{\times}10^5$m/s, $\Delta^{CB}$= 0.1 eV, $m^{*CB}$ = 0.6 $m_e$, $a_0^{CB}$ = 0.05 eV, $a_3^{CB}$ = 0.1i eV, $a_1^{CB}, a_2^{CB}$ = 0. Similarly, $\Delta^{VB}$= -0.02 eV, $m^{*CB}$ = -0.9 $m_e$, $a_0^{VB}$ = 0.03 eV, $a_3^{VB}$ = 0.05i eV, $a_1, a_2 = 0$

$$H(k) = \begin{pmatrix} H_{Dirac} & V_{int} \\ V_{int}^{\dagger} & H_{defect,QW} \end{pmatrix}. \tag{1}$$

The hamiltonians for Dirac states, and defect and Quantum Well (QW) states are given as

$$H_{Dirac} = v_F \hbar (k \times \sigma) \cdot \hat{z}, \tag{2}$$

$$H_{defect,QW} = \begin{pmatrix} H_{defect} & I_{2\times2} \cdot 0 \\ I_{2\times2} \cdot 0 & H_{QW} \end{pmatrix}. \tag{3}$$

Here, $k$ is the wave-vector and $v_F$ is the Fermi velocity.

$$H^x = (\frac{\hbar^2 k^2}{2m^{*x}} + \Delta^x) \cdot I_{2\times 2}, \tag{4}$$

here, $H^x$ is the hamiltonian for the, $x$ = defect/QW state. $m^*$ is the effective mass of the electrons in the defect/QW states and $\Delta$ is the shift of the parabola with respect to the Dirac point.

$$V_{int}^x = a_0^x \cdot I_{2\times 2} + a_1^x \cdot \sigma_1 + a_2^x \cdot \sigma_2 + a_3^x \cdot \sigma_3. \tag{5}$$

Where, $V_{int}$ is the interaction with the defect/QW states in the $x$ = valence band (VB) or conduction band (CB). $\sigma_i$ are the Pauli spin matrices and $a_i$'s are the coefficients, where $a_0$ is strictly real and $a_i$, i=1 to 3 are strictly imaginary for time reversal symmetry preserving interaction.

$$V_{int} = \begin{pmatrix} V_{int}^{CB} & V_{int}^{VB} \end{pmatrix}_{4\times 2}. \tag{6}$$

# S8 Spin-momentum locking plots

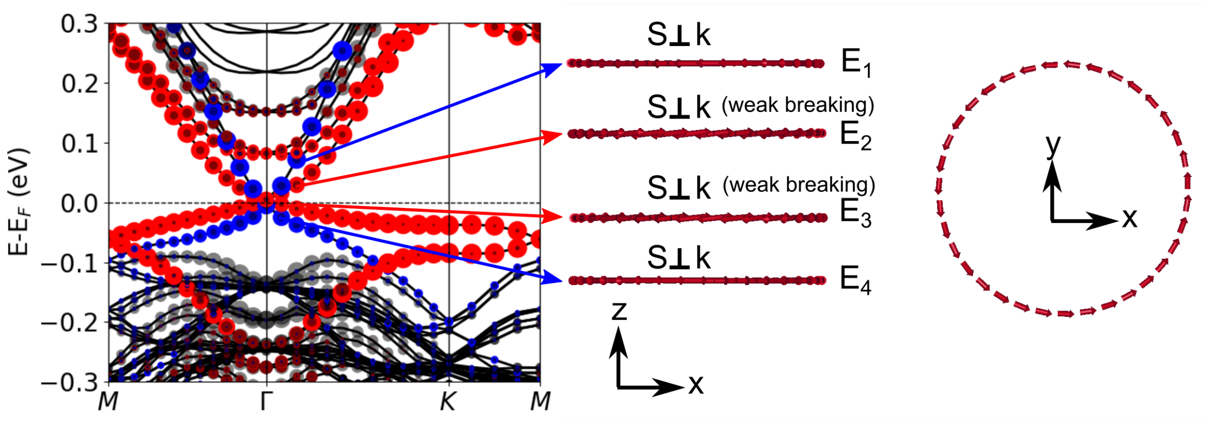


Figure S11: The in-plane projection of the spin at energies $E_1$ to $E_4$ for blue (bottom surface) and red (top surfaces) bands, for 5×5×7 QL with a single Se vacancy at the top surface.

We find that for the hybrid (defect + top surface state) topological band (in red at $E_2$), the spin-momentum locking is very weakly disturbed. This is mostly on account of the high in-plane concentration of the defect. Nevertheless, the preservation of the spin-momentum locking even in the presence of defects is the signature of topological protection of the surface states.

## S9 Depolarizing field across the defective slab

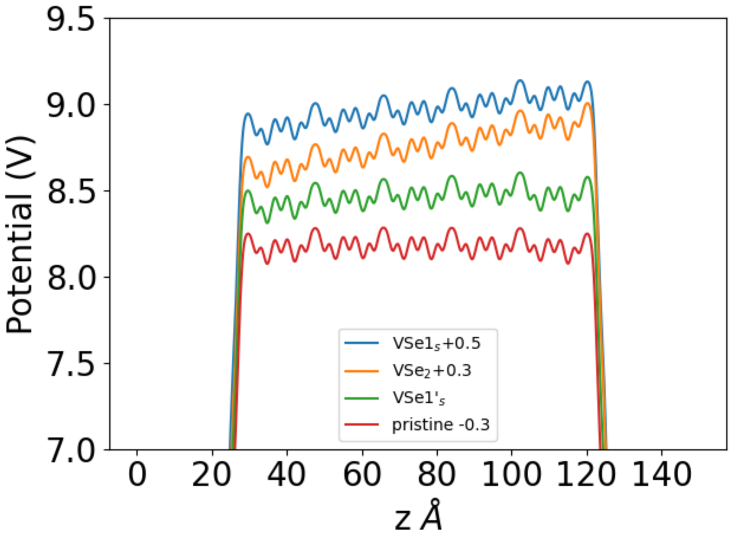


Figure S12: The macroscopically averaged electric potential experienced by electrons across the 6×6×1 QLs slab with surface vacancies. The potential curves, which otherwise overlap, are shifted with respect to each other for sake of clarity.

Figure S12 shows that the largest gradient of the potential across different layers (i.e. depolarizing field) is for VSe2$_s$ defect on the top surface. The gradient of the potential can be correlated to the shift of the lower surface state into the valence band (see main text), with VSe2$_s$ showing the largest shift. This depolarizing field causes a tiny fraction of electrons to move into the bottom QL, which results in the n-doping of the bottom QL, shifting the Dirac cone associated with the bottom layer below the Fermi level (see main text Figure 4 A). This is followed by VSe1$_s$, which shows the exact same behavior, but with smaller magnitude. However in the case of VSe1$_s$', the potential profile across the layers resembles that of pristine layer. As VSe1$_s$'is at the interface of two layers, we attribute its potential profile to the effective screening of the charges in the n-doped top QL by the adjacent QL, which significantly reduces the depolarizing field across the slab. Hence, there is no significant charge transfer into the bottom QL from the top QL, and consequently the splitting between the hybrid defect state and the bottom Dirac state is negligibly small (see main text Figure 3 C).

## S10 Rashba splitting in $VSe_1$

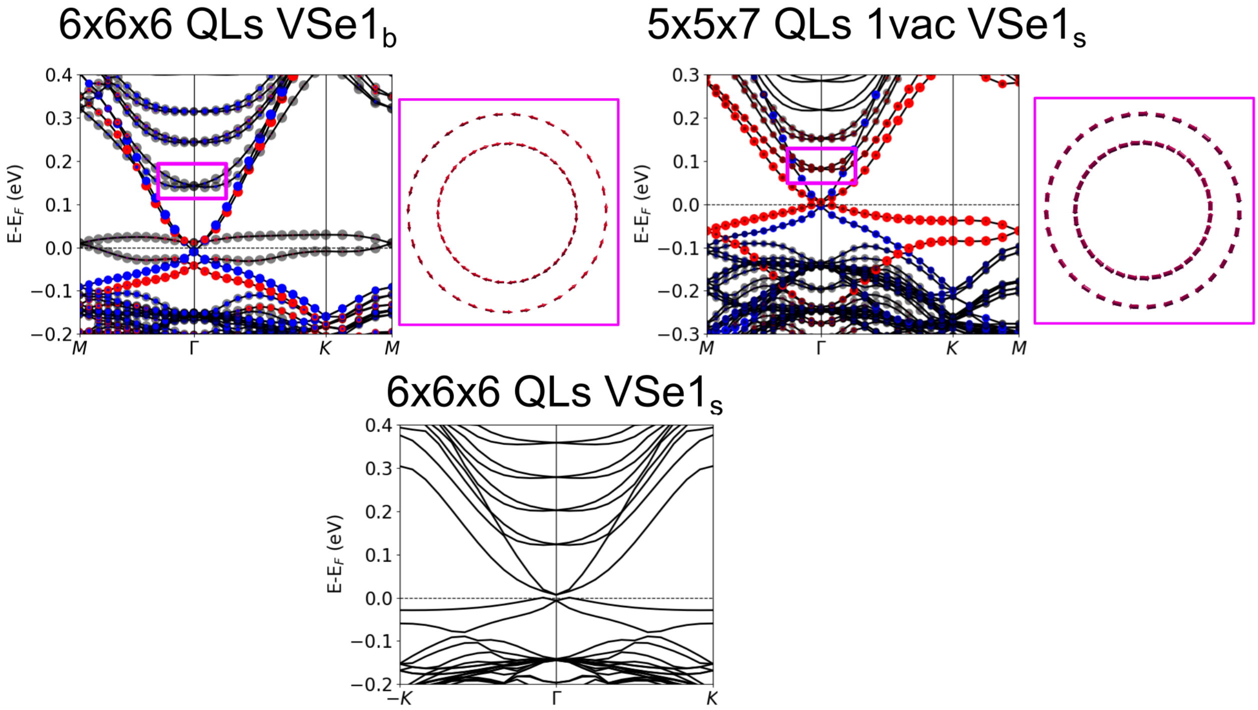


Figure S13: Top row: Spin-texture plots showing Rashba splitting in surface and bulk vacancies. Bottom row: Electronic band structure for $VSe_1$ in 6×6×1 QL slab along -K −Γ− K. Note the Rashba-like splitting of the conduction band states.

# S11 Convergence plots

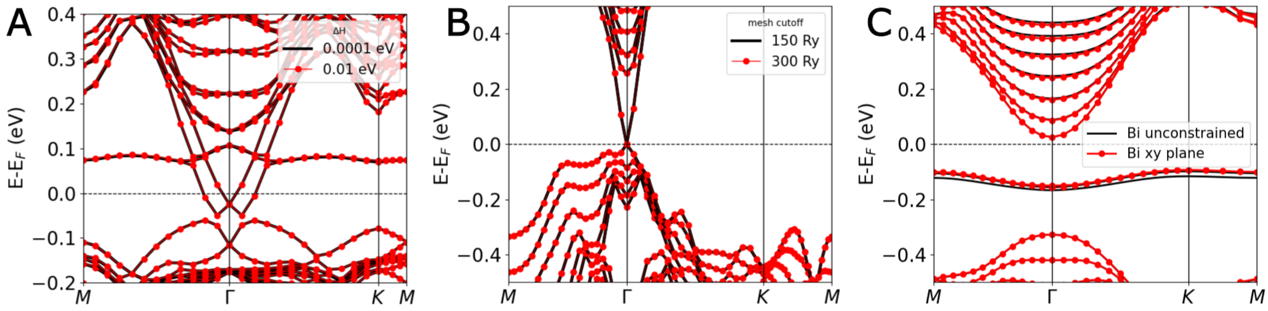


Figure S14: Convergence studies for electronic band structure: A) VSe2$_b$ with different convergence criteria for self-consistency in the Hamiltonian (H) matrix elements in 6×6×6 QL slab. B) Pristine 1×1×6 QL with different plane wave mesh cutoffs (300 Ry and 150 Ry). C) VSe1$_s$ in 5×5×7 QL slab with Bi atoms adjacent to vacancy are allowed to move in-plane and unconstrained but without spin-orbit coupling.

We carried out convergence studies with respect to plane wave energy mesh cutoffs and maximum absolute change in the Hamiltonian matrix elements to check the convergence of the electronic structure properties. The results of different convergence tests are summarized in Figure S14 A and B, showing that our adopted energy cut-offs and energy convergence criterion are robust and we can safely say that the calculations are converged. In addition, we also tested the change in structure and electronic bands imposed by Bi atoms being constrained to move only in-plane (xy-plane). Here, we let the Bi atoms next to the vacancy to relax freely without any constraint and found that it weakly breaks the symmetry. Hence, our calculations keeping the Bi atoms constrained to move only in xy-plane is a reasonable assumption, which provides reasonably-accurate results, while making the calculations on large supercells tractable.

# S12 $VSe1_s$ in 3×3×7, 5×5×7 and 6×6×6 QL slabs

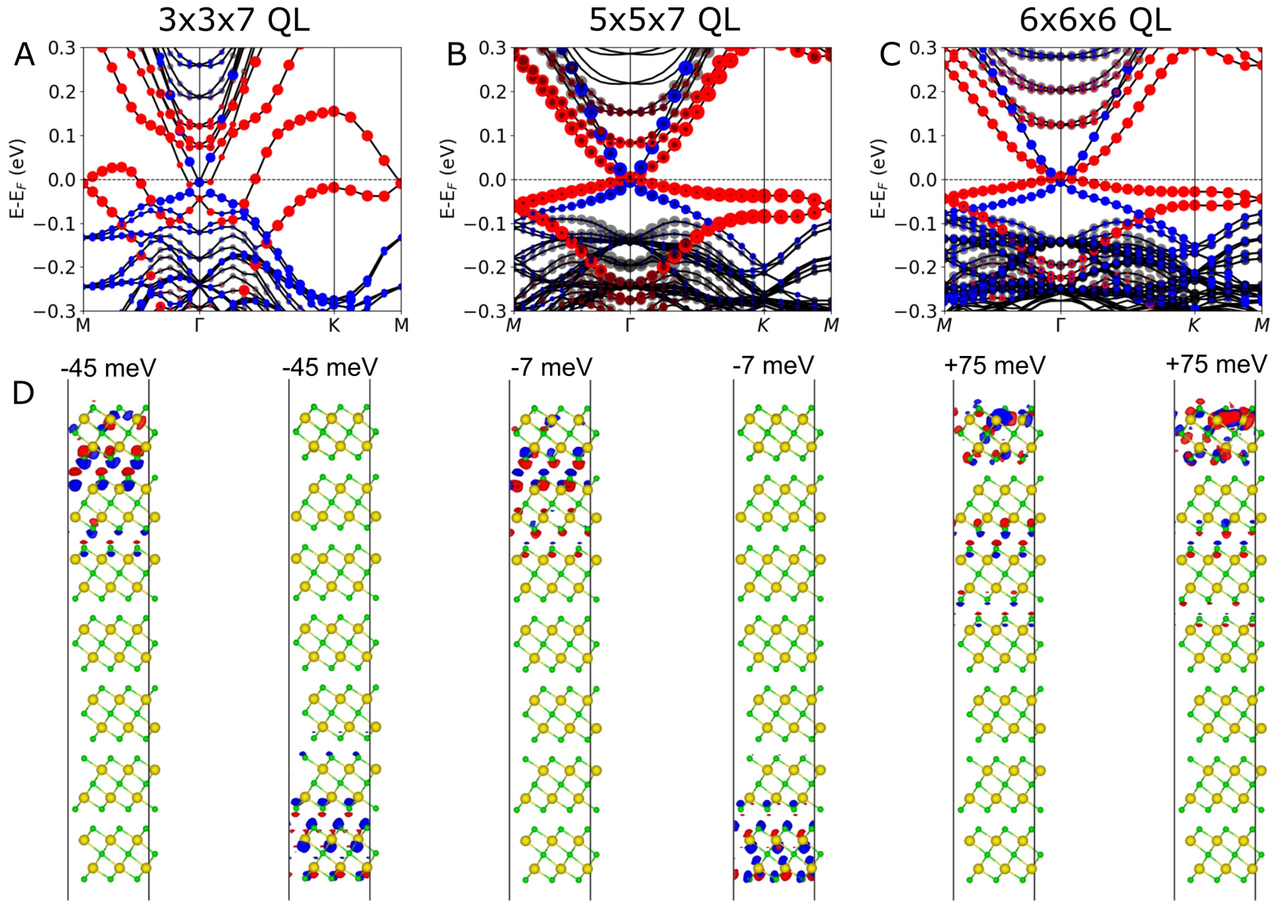


Figure S15: Comparison of electronic structure with varying surface concentration (by varying the in-plane size of the supercell) of single $VSe1_s$. A) 3×3×7 QL, B) 5×5×7 QL and C) 6×6×6 QL slab each have 1 Se vacancy on the top surface. Color scheme, red: top QL contribution, blue: bottom QL contribution and black: bulk contribution to the electronic states. D) Wavefunctions of $VSe1_s$ in 3×3×7 QL slabs at the Γ-point in the BZ. The energy of the state with respect to Fermi level is indicated above the respective wavefunction plots. Color scheme, Se: green and Bi: yellow.

The effect on surface concentration of single Se vacancies is shown in Figure S15. The surface density for the slabs corresponds to $8\times10^{13}$ cm$^{-2}$, $3\times10^{13}$ cm$^{-2}$ and $2\times$ $10^{13}$ cm$^{-2}$ in 3×3×7 QL, 5×5×7 QL and 6×6×6 QL slabs, see Figure S4 and Figure 3 in main text, respectively. Most noticeably, we find that for the smallest in-plane supercell (i.e. 3×3×7 QL slab), the bands at the Fermi level are considerably distorted and impart metallicity to the configuration [9]. On the other hand, the interaction between the periodic images of $VSe1_s$ in 5×5×7 QL and 6×6×6 QL slabs is almost the same. This can be inferred from the bands at the Fermi level which become flatter as compared to those in the 3×3×7 QL slab, and show similar dispersion. Again, the magnitude of shifting of the top layer's surface state (Dirac cone) into the valence band increases with increasing concentration of the in-plane defect density. As we can see, the shifting energies are $<$ -300 meV, -275 meV, and -225 meV for A), B) and C) in Figure S15, respectively. It is non-trivial to project from this data, but one could surmise that

the shift of the top surface state should reach a value close to the Fermi level for a single defect in an infinite slab [10, 11]. A closer inspection of the wavefunctions for the 3×3×7 QL slab near the Fermi level, reveals a stark difference with those in the other two concentrations (see Figure S5 in SI and Figure 3 in main text). We find that due to the high defect concentration, the defect state mixes strongly with the surface state associated with the top layer.

## References


[1] L. A. Walsh *et al.*, ACS Nano **12**, 6310 (2018), pMID: 29874037.

[2] G. M. Stephen *et al.*, The Journal of Physical Chemistry C **124**, 27082 (2020).

[3] A. Pertsova and C. M. Canali, New Journal of Physics **16**, 063022 (2014).

[4] D. Hsieh *et al.*, Nature **452**, 970 (2008).

[5] P. D. C. King *et al.*, Phys. Rev. Lett. **107**, 096802 (2011).

[6] M. Bianchi *et al.*, Nature Communications **1**, 128 (2010).

[7] T. V. Menshchikova, S. V. Eremeev, and E. V. Chulkov, JETP Letters **94**, 106 (2011).

[8] L. Seixas, D. West, A. Fazzio, and S. B. Zhang, Nature Communications **6**, 7630 (2015).

[9] S. Wang and P. Zhang, Physics Letters A **384**, 126281 (2020).

[10] L. Miao *et al.*, npj Quantum Materials **3**, 29 (2018).

[11] M. Zhong *et al.*, Scientific Reports **7**, 3971 (2017).
